# Supplementary material for: From Engineering Diagrams to Graphs: Digitizing P&IDs with Transformers
Source: arXiv:2411.13929 source file (2025-12-19)

## Modular Digitization Approach

## Predicted Bounding Boxes

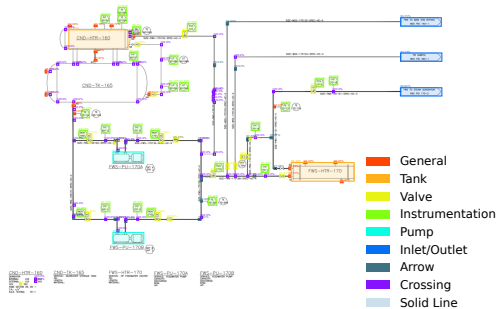

### Predicted Graph

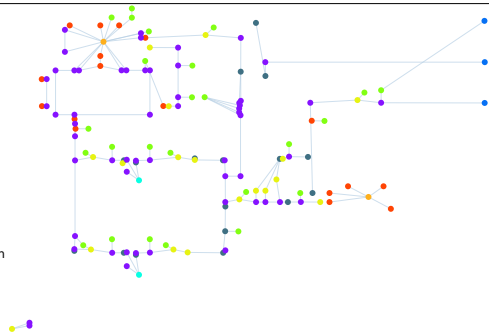

## Relationformer

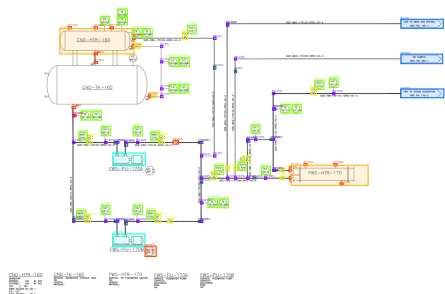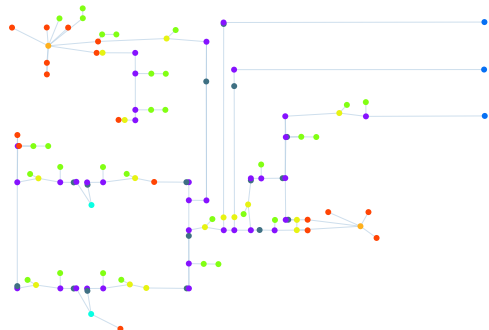

Supplement: Supplementary file 1 [file whole_plan_prediction_3_both.pdf]
