# Supplementary material for: From Engineering Diagrams to Graphs: Digitizing P&IDs with Transformers
Source: arXiv:2411.13929 source file (2025-12-19)

Modular Digitization Approach

Predicted Bounding Boxes

Predicted Graph

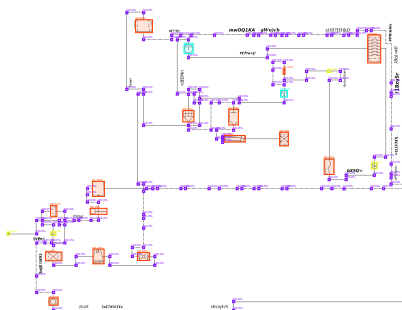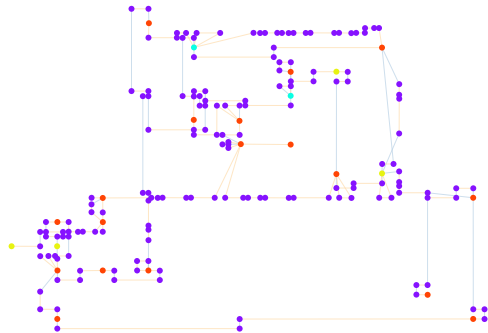

Relationformer

- General
- Tank
- Valve
- Instrumentation
- Pump
- Crossing
- Solid Line
- Non-Solid Line

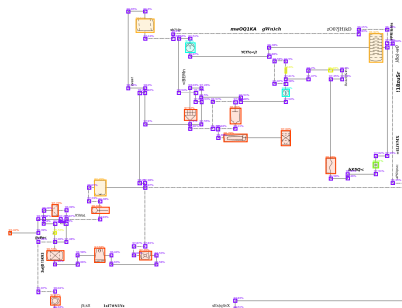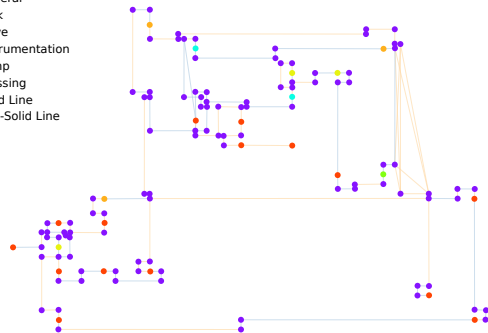

Supplement: Supplementary file 2 [file whole_plan_prediction_synth_0_both.pdf]
